# Supplementary material for: Humans Are Easily Fooled by Digital Images
Source: arXiv:1509.05301 source file (2015-09-17)
Supplement: Supplementary file 1 [file appendix.tex]

\appendices

\section{Image Difficulty}

\begin{figure}[ht]
  \centering
  \includegraphics[width=3in]{images/percentDifficultyReal}
  \caption{Distribution of answers classes per image based on image difficulty for real images.}
	\label{fig:percentDifficultyReal}
\end{figure}

\begin{figure}[ht]
  \centering
  \includegraphics[width=3in]{images/percentDifficultyFake}
  \caption{Distribution of answers classes per image based on image difficulty for fake images.}
	\label{fig:percentDifficultyFake}
\end{figure}

One of the main objectives of our test was to answer the question: "What features of an image can make it harder for an user to find manipulation in it?". The hit rate for each image is a starting point for this evaluation, but it is not sufficient to answer our questions. In this session, we showed that the variation in color in an image (Variance feature) can be related with performance, time, confidence and use of hints, suggesting that high variation in color makes an image harder to visually inspect. 

Instead of asking the users directly their opinion, we formulate a metric to assess image difficulty using the provided features for each answer. This metric is subjective and relative to a closed set of images in our test, and it substitutes the question: "Between each of these images, which ones were harder?". The reasoning behind the formula is based on the following assumptions:

If an user guessed the image right:
\begin{itemize}
\item The lower the confidence in the answer, the harder the image is. If the image left the user uncertain in his answer, it could be considered harder.
\item The longer the user took to answer, the harder the image is.
\item If the user asked for a hint, the image is harder than another one were he did not ask for a hint.
\end{itemize}

However, if the user guessed the image wrong:
\begin{itemize}
\item The higher the confidence in the answer, the harder the image is. The user guessed the image wrong, therefore the more confident he was, the more fooled he was by the image, and consequently it can be considered harder.
\item If the user answered too quickly, it is possible that the was fooled quickly and the image is hard. However, if he took too much time to answer, it could also mean it is a hard image to answer. In this sense, the more the answer time deviates from the average, the harder the image is.
\item If the user asked for a hint, the image is harder than another one were he did not ask for a hint.
\end{itemize}

Consider $\Omega$ as the set of all answers, $\Omega(i)$ as the subset of answers to the image $i$ and $\Omega(i,a)$ a specific answer $a$ represented as a vector in the form $[r,c,t,h]$. In this case, $r$ represents if the answer is right, assuming values in the set $\{0,1\}$, $c$ represents the answer confidence, assuming values in the set $\{1,2,3\}$, $t$ is a real scalar greater than zero representing answer time and $h$ indicates if a hint was asked for image, also in the set $\{0,1\}$. We can then summarize the image difficulty function $I_d(i)$ as the average of the answer difficulty function $A_d$ for all answers in $\Omega(i)$:

\begin{equation}
I_d(i)=\sum_{a=1}^{n}\frac{A_d(\Omega(i,a))}{n}
\end{equation}

\begin{equation}
A_d(r,c,t,h)=\begin{cases}
  c+\tau(r,t)-\beta h, & \mbox{if } r = 1 \\
  -c+\tau(r,t)-\beta h,  & \mbox{if } r = 0 
\end{cases}
\end{equation}

The function $\tau(r,t)$ weight the time influence on difficulty when the answer is right or wrong, respectively. It uses the global mean $\mu_t$ for all answer times and the standard deviation $\sigma_t$:

\begin{equation}
\tau(r,t) =\begin{cases}
  -\frac{1}{\sigma \sqrt{2\pi} } e^{ -\frac{(x-\mu_t)^2}{2\sigma_t^2} }, & \mbox{if } r = 1 \mbox{ and } t <\mu_t  \\
  \frac{1}{\sigma \sqrt{2\pi} } e^{ -\frac{(x-\mu_t)^2}{2\sigma_t^2} },  & \mbox{otherwise}
\end{cases}
\end{equation}

After estimating the difficulty for all images, they are normalized from [0,1], where 0 is the easiest image and 1 is the hardest. 

\begin{figure}[ht]
  \centering
  \includegraphics[width=3in]{images/timeFuncR}
  \caption{Difficulty function for time in right answers. Note that the graph is wrong and should be from -100 to 100.}
	\label{fig:timeFuncR}
\end{figure}

\begin{figure}[ht]
  \centering
  \includegraphics[width=3in]{images/timeFuncW}
  \caption{Difficulty function for time in wrong answers. Note that the graph is wrong and should be from -100 to 100.}
	\label{fig:timeFuncW}
\end{figure}

\section{Drafts and Graph Dumps}
\label{sec:Drafts}

This section is a temporary dump of graphics for quick evaluation.

\subsection{Age}

\begin{figure}[ht]
  \centering
  \includegraphics[width=3in]{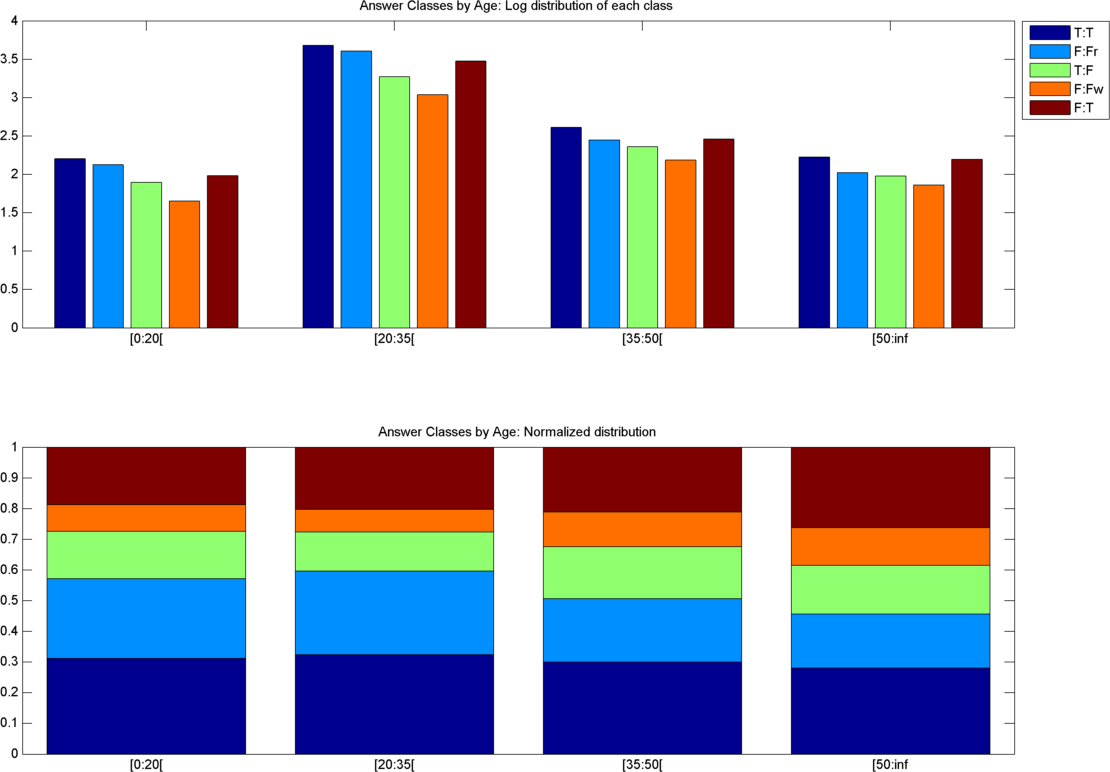}
  \caption{Distribution of answer classes per age.}
	\label{fig:percentAge}
\end{figure}

Figure. ~\ref{fig:percentAge}: The most clear aspect of this graph is the decay of the right answers rate with age and the increasing of the F:T answer class, meaning that older age groups are less likely to perceive forgery in an image. 

The performance peaks at the young adult interval of [20,35[, followed by the teenager group aged [0,[20. The most likely reasons for this are:

\begin{enumerate}
	\item Younger individuals tend to have better visual acuity. 
  \item The younger age groups have grown with a better access to technology and generally have more contact with digital images.
	\item Teenagers are less mature, and therefore less likely to commit to the test than young adults.
	\item Teenagers generally will have less experience than young adults.
\end{enumerate} 

It must be noted, however, that the great majority of answers is concentrated on the two central intervals between [20,50[, having thousands of answers while the interval [0:20[U[50:inf[ has hundreds of answers.

\subsection{Education}

\begin{figure}[ht]
  \centering
  \includegraphics[width=3in]{images/percentEducation}
  \caption{Distribution of answer classes per education.}
	\label{fig:percentEducation}
\end{figure}

Figure. ~\ref{fig:percentEducation}: there was little to no correlation between education and performance, and the vast majority of answers were done by people with at least some college education.

\subsection{Experience}

\begin{figure}[ht]
  \centering
  \includegraphics[width=3in]{images/percentExperience}
  \caption{Distribution of answer classes per experience.}
	\label{fig:percentExperience}
\end{figure}

Figure. ~\ref{fig:percentExperience}: there is some improvement on performance due to user experience with digital images. The overall difference from user experience to profession amounts to about 10\%. There was only a single, invalid user with no experience at all in digital images.

Analyzing together performance based on user background, age seems to play the larger role, followed by experience with digital images while education matters little. One important point is that the majority of users are young adults and we have a large number of answers by both amateurs and professionals, which are one of the best performing categories. If we can assert that there is correlation between experience, age, and performance, and a large part of our sample pool is of the best suited users to detect forgery (young adults with professional experience on digital images), it is probable that the general population would fare worse on the test. Since our overall performance is already low (circa 55\%), it makes our point that humans are easily fooled stronger.

\subsection{Time}

\begin{figure}[ht]
  \centering
  \includegraphics[width=3in]{images/percentTime}
  \caption{Distribution of answer classes per Time.}
	\label{fig:percentTime}
\end{figure}

Figure. ~\ref{fig:percentTime}: the most visually striking statistic perceived in this graph is that the chance of saying a false image is true decreases greatly the more time you spend looking at it, while increasing the chance of saying a true image is fake. The three central classes displayed in the graph represent answers where the user said the image was false, and it only increases overall. This means that if you look at an image for too long, you are probably going to say it is fake. 

The mean time is in the interval [20:40] seconds, which is the mininum necessary for asking for a hint. This interval also is the one with the larger absolute amount of right answers. 

\subsection{Full Resolution}
\label{sec:Fullres}

\begin{figure}[ht]
  \centering
  \includegraphics[width=3in]{images/percentFullRes}
  \caption{Distribution of answers classes based on if the user clicked on the full resolution image or not.}
	\label{fig:percentFullRes}
\end{figure}

Figure. ~\ref{fig:percentFullRes}: the majority of answers was done without checking the full resolution image. That being said, seeing the image in full resolution results in a slight increase (2\%) of performance. The most interesting aspect of this graph is that by seeing the full resolution images, users were less inclined to say a false image was true and more inclined to say a true image was false. For right answers, the increase seems to be mostly on guessing the true images right. Furthermore, if we consider the amount of answers to true images in both cases (classes 1+3), we can notice that it changes from 44.5\%, which is the same proportion in the image pool, to almost 51\%, meaning people are opening more often true images. 

It is not completely clear what this all could mean in conjunction. My guess would be that most of the times images with less visual clues to adulteration force the user to open them in full resolution. Since true images contain no actual adulteration, users tend to open them in full resolution to do a harder check. In other words, opening the image in full resolution is not necessarily changing the answering behavior, but a particular set of images, which are mostly true, are making users consult them in full resolution.

Another possible explanation is that there is a particular answering behavior of users who consistently view images in full resolution, while others don't. In this sense, the right graph is comparing the answer distribution for this set of users, when they clicked in the full resolution images, to the rest of the answer pool.

\subsection{Hints}

\begin{figure}[ht]
  \centering
  \includegraphics[width=3in]{images/percentHint}
  \caption{Distribution of answers classes based on if the user asked for a hint or not.}
	\label{fig:percentHint}
\end{figure}

Figure. ~\ref{fig:percentHint}: Firstly and most importantly, it must be noted that the performance decreased (59\% to 55\%) when the user asked for a hint. This probably means that users ask for a hint when they really do not know the answer, since they already had at least 20 seconds to look at the image in the first place. The proportion of answers to a real image also changes from 43\% to almost 52\%, reinforcing the argument from Section.~\ref{sec:Fullres} that true images force users to look harder.

\subsection{Type}

\begin{figure}[ht]
  \centering
  \includegraphics[width=3in]{images/percentType}
  \caption{Distribution of answers classes based on image type.}
	\label{fig:percentType}
\end{figure}

Figure. ~\ref{fig:percentType}: this graph shows that people tend to guess right true images most of the time (around 70\%), while the hardest type of forged images to guess are erasing, copy-pasting and splicing, in this order. For forged images, this is also the order of image types with more amount, with 20 for erasing, 35 to copy-paste and 42 to splicing. This difference could account for some of the change in performance, but not all, so we must do a bootstraping check on the future.

\subsection{Confidence per Image}

\begin{figure}[ht]
  \centering
  \includegraphics[width=3in]{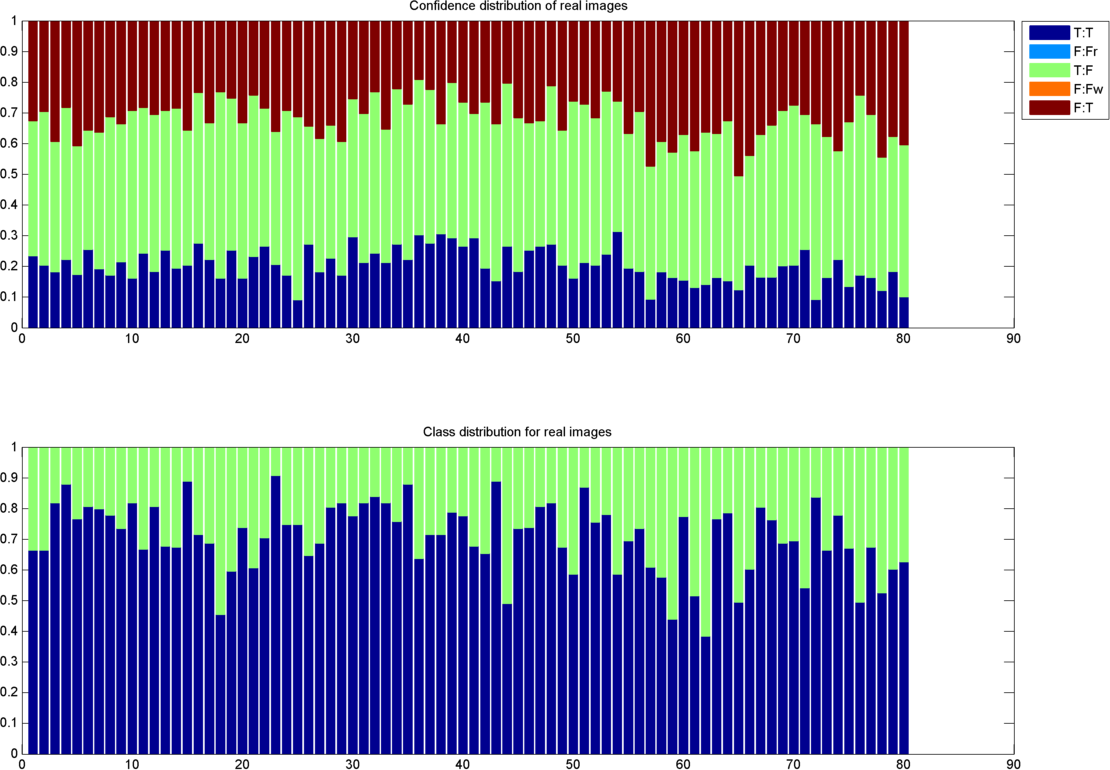}
  \caption{Distribution of answers classes per image based on answer confidence for real images.}
	\label{fig:percentConfidenceReal}
\end{figure}

\begin{figure}[ht]
  \centering
  \includegraphics[width=3in]{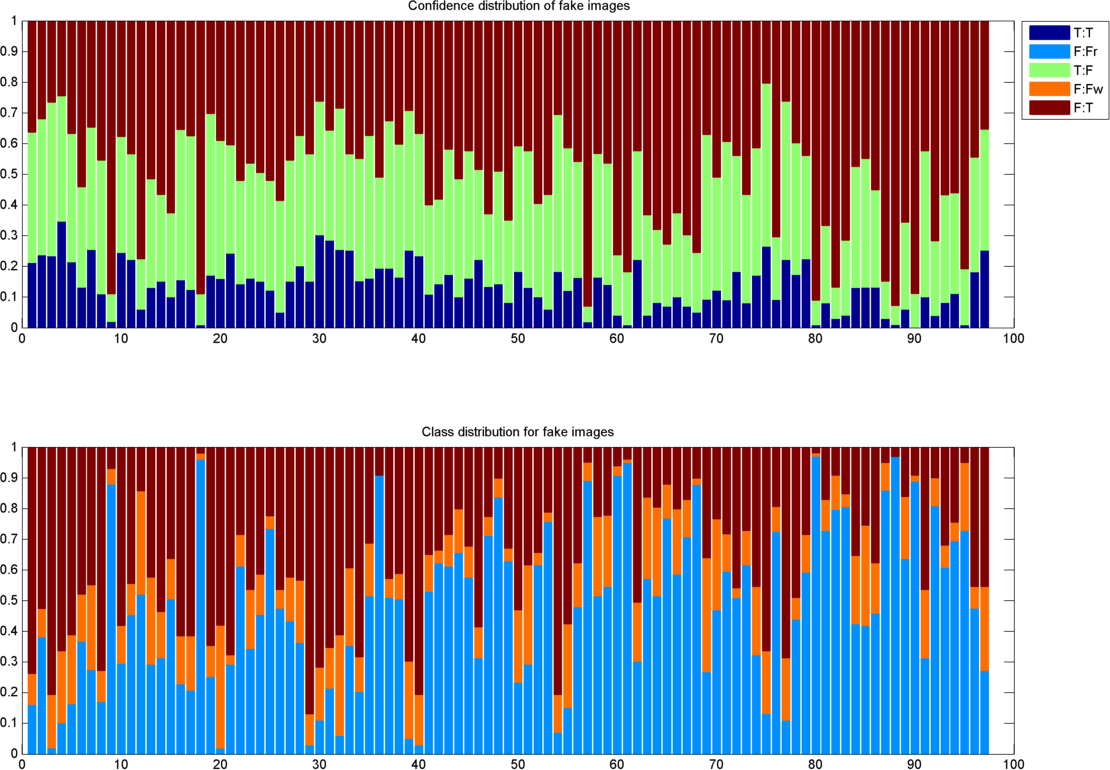}
  \caption{Distribution of answers classes per image based on answer confidence for fake images.}
	\label{fig:percentConfidenceFake}
\end{figure}

Figures \ref{fig:percentConfidenceReal} and \ref{fig:percentConfidenceFake}: these images might be a bit confusing at first because of the coloring and the legend, but they are easy to understand. In the bottom, we have the class distribution of answer as seen in all other examples, but in one image only for real images and in the other for the fake images. On the top, we have a similar display per image, but indicating distribution of confidences. In this case, dark blue indicates low confidence, green indicates medium confidence and brown high confidence.

These graphs represent the same information displayed in Figure. ~\ref{fig:percentConfidence}, but without being condensed. In this sense, the brown class on top is analogous to the light blue on the bottom, because high confidence answers usually got were right on fake images.

\subsection{Time per Image}

\begin{figure}[ht]
  \centering
  \includegraphics[width=3in]{images/percentTimeReal}
  \caption{Distribution of answers classes per image based on answer time for real images.}
	\label{fig:percentTimeReal}
\end{figure}

\begin{figure}[ht]
  \centering
  \includegraphics[width=3in]{images/percentTimeFake}
  \caption{Distribution of answers classes per image based on answer time for fake images.}
	\label{fig:percentTimeFake}
\end{figure}

Figures \ref{fig:percentTimeReal} and \ref{fig:percentTimeFake}: i did not dedicate too much time for this image, but it seems to comply with the results from the overall time evaluation.

\subsection{Edited Area per Image}

\begin{figure}[ht]
  \centering
  \includegraphics[width=3in]{images/editedAreaxClasses}
  \caption{Distribution of answers classes per image based on the edited area for the image, on ascending order.}
	\label{fig:editedAreaxClasses}
\end{figure}

An important aspect to be analyzed is if the size of the edited area on an image has a great impact on its error rate. It is intuitive to think that the larger the portion of the image is edited, it is most likely for it to be perceived. Fig.~\ref{fig:editedAreaxClasses} shows that this is not true. By dividing the edited area from the ground truth masks by the total image area we can obtain the portion of the image that has undergone change. Ordering these values per image, and relating them to the answer classes for the fake images reveals no correlation. 

This corroborates with the observed results that hints, which reduce the evaluation area for images, do not have a significant impact on performance overall. 
